# Supplementary material for: A simple and effective predictive resource scaling heuristic for large-scale cloud applications
Source: arXiv:2008.01215 source file (2020-08-03)
Supplement: Supplementary file 1 [file appendix.tex]

% !TEX root = resources_scaling.tex
\section{Data sets} \label{sec:datasets}

\subsection{Artificial data generation} \label{subsec:data-generation}

Both artificial data sets were generated using the GluonTS toolkit. More specifically,
\begin{itemize}
	\item
	$D_2$ was generated using `ComplexSeasonalTimeSeries` with the following parameters: blabla
	\item
	$D_3$ was generated through the general `RecipeDataset` class with the following recipe details: blabla
\end{itemize}

\subsection{More plots}

\begin{figure}[!htb]
  \begin{subfigure}[t]{1\textwidth}
    \centering
	\includegraphics[width=0.32\linewidth]{./figures/data/datasets/artificial/easy/test/_1.pdf}
	\includegraphics[width=0.32\linewidth]{./figures/data/datasets/artificial/easy/test/_2.pdf}
	\includegraphics[width=0.32\linewidth]{./figures/data/datasets/artificial/easy/test/_3.pdf}
    \caption{Easy artificial data samples}
  \end{subfigure}

  \medskip

  \begin{subfigure}[t]{1\textwidth}
    \centering
	\includegraphics[width=0.32\linewidth]{./figures/data/datasets/artificial/hard/test/_4.pdf}
	\includegraphics[width=0.32\linewidth]{./figures/data/datasets/artificial/hard/test/_6.pdf}
	\includegraphics[width=0.32\linewidth]{./figures/data/datasets/artificial/hard/test/_8.pdf}
    \caption{Hard artificial data samples}
  \end{subfigure}

  \medskip

  \begin{subfigure}[t]{1\textwidth}
    \centering
	\includegraphics[width=0.32\linewidth]{./figures/data/datasets/icc/test/_1.pdf}
	\includegraphics[width=0.32\linewidth]{./figures/data/datasets/icc/test/_2.pdf}
	\includegraphics[width=0.32\linewidth]{./figures/data/datasets/icc/test/_3.pdf}
    \caption{Real traffic data samples}
  \end{subfigure}
  \caption{title}
\end{figure}

\newpage

\section{GluonTS forecasting models details}

We provide here some details about the predictive models that were used to forecast the traffic.

\paragraph{Hyper-parameters}

blabla

\newpage

\section{Results}

blabla
